# Supplementary material for: Bridging the Gap: Enhancing the Utility of Synthetic Data via Post-Processing Techniques
Source: arXiv:2305.10118 source file (2023-06-06)
Supplement: Supplementary file 1 [file supplementary.tex]

\newpage
\section*{GAN Architecture}
% As generative model architecture, we decided to use BigGAN Deep. Specifically, we chose to adopt the implementation proposed in \textit{StudioGAN} library\footnote{\url{https://github.com/POSTECH-CVLab/PyTorch-StudioGAN/}}, which makes some minor changes in the layout of layers of the residual blocks of the generator and discriminator. Namely, in the $G$ block, instead of dropping channels, the residual path is first upsampled and then a \textit{Conv1x1} is applied to ensure that the number of channels between the two paths, residual and non-residual, is the same. Similarly, In the $D$ block, the residual path is first passed through a \textit{Conv1x1} to output the correct number of channels and then is downsampled. Figure~\ref{fig:proposed_pipeline} provides a comparison between the original version and the StudioGAN implementation of the BigGAN Deep blocks.
We employed the BigGAN Deep architecture as our generative model. Specifically, we utilized the implementation from the \textit{StudioGAN} library\footnote{\url{https://github.com/POSTECH-CVLab/PyTorch-StudioGAN/}}, which introduces slight modifications to the layout of residual blocks in both the generator and discriminator. In the generator's $G$ block, rather than dropping channels, we upsample the residual path and apply a \textit{Conv1x1} operation to ensure consistent channel numbers between the residual and non-residual paths. Similarly, in the discriminator's $D$ block, we first pass the residual path through a \textit{Conv1x1} layer to obtain the correct channel output and then downsample it. For a visual comparison of the original BigGAN Deep blocks and the StudioGAN implementation, refer to Figure~\ref{fig:proposed_pipeline}.

\begin{figure}[!h]
    \vspace{-10pt}
    \centering
    \includegraphics[width=1.\textwidth]{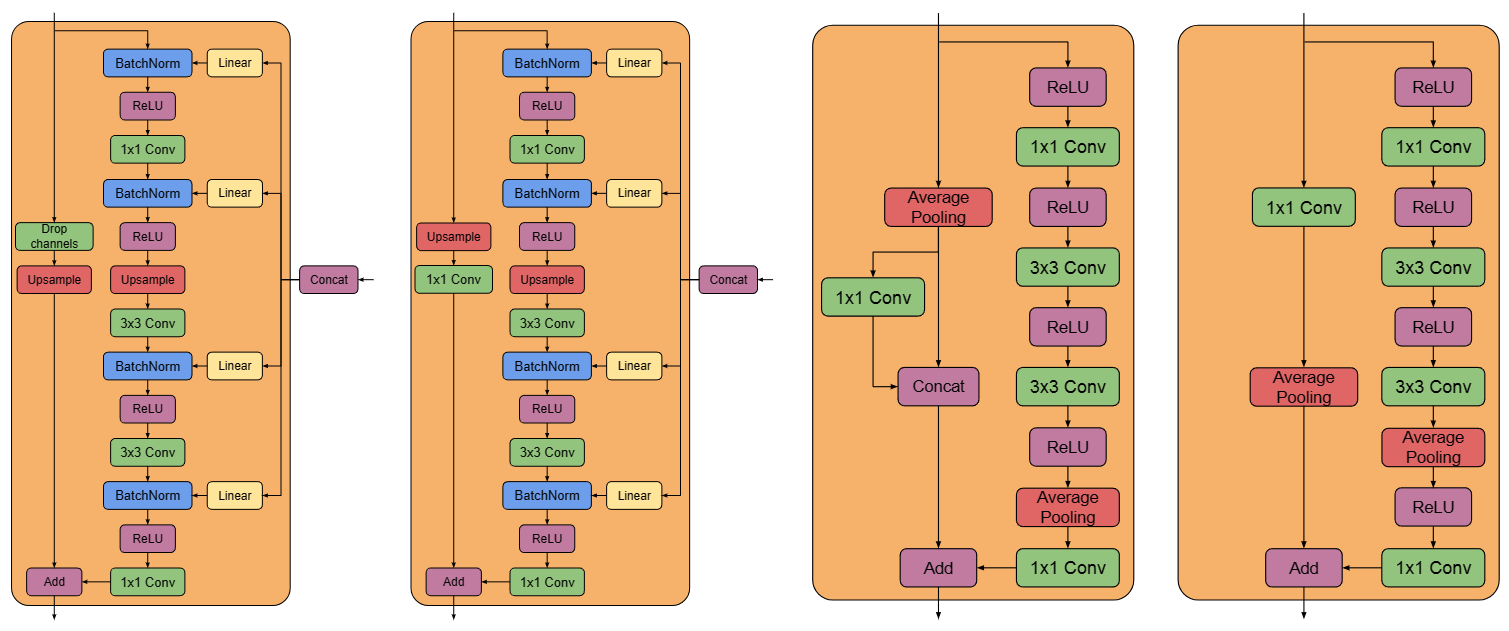}
    \caption{BigGAN Deep blocks architectures. From left to right, the legacy Generator block, the StudioGAN Generator block (used in our work), the legacy Discriminator block, the StudioGAN Discriminator block (used in our work).}
    \label{fig:proposed_pipeline}
\end{figure}

% All the models are trained for 500 epochs with batch size 192, using 3 $D$ steps per $G$ step. Our interpretation of \textit{“$N$ $D$ steps per $G$ step”} is slightly different to that used into its original formulation, but we have found experimentally that it gives better results. Specifically, instead of splitting the batch (i.e., size 192) into $N$ sub-batches (i.e., size 64) and training the discriminator on each of these, we train $N$ times $D$ on the whole big batch (i.e., size 192) (see Figure~\ref{fig:discrimination_steps_legacy_vs_ours}). We hypothesize that this modification may give better results on smaller datasets than ImageNet, which is the same reason why we do not adopt large batch sizes (2048) as proposed by the authors of BigGAN, who train the model on ImageNet. Lastly, we employed only random horizontal flip as the sole form of data augmentation for the training set.
All models underwent training for 500 epochs, employing a batch size of 192 and utilizing 3 discriminator ($D$) steps per generator ($G$) step. While our interpretation of "N $D$ steps per $G$ step" differs slightly from its original formulation, our experimental findings have shown that it leads to superior results. Specifically, instead of dividing the batch (size 192) into N sub-batches (size 64) and training the discriminator on each sub-batch, we perform N iterations of discriminator training on the complete batch (size 192) (refer to Figure~\ref{fig:discrimination_steps_legacy_vs_ours}). We conjecture that this modification may yield improved outcomes on datasets smaller than ImageNet, which is why we refrain from adopting the larger batch sizes (2048) proposed by the authors of BigGAN, who trained the model on ImageNet. Lastly, our training set only employed random horizontal flips as the sole form of data augmentation.

\begin{figure}[!h]
    \vspace{-10pt}
    \centering
    \includegraphics[width=0.45\textwidth]{images/Discrimination Steps - Traditional.pdf}\hfill
%\quad
    \includegraphics[width=0.45\textwidth]{images/Discrimination Steps - Ours.pdf}\hfill
    \caption[Discrimination Steps - Legacy Vs Ours]{Discrimination Steps - Legacy Vs Ours.}
    \label{fig:discrimination_steps_legacy_vs_ours}
\end{figure}

\newpage
\section*{Dynamic Sample Filtering}

The relationship between the filtering threshold of the Dynamic Sample Filtering technique and the discarded image count, leading to a balanced dataset size of 50,000 images, is illustrated in Figures~\ref{fig:filterfmnist},~\ref{fig:filtercifar10}, and~\ref{fig:filtercifar100}. Notably, the results demonstrate that for the \textit{Fashion-MNIST} and \textit{CIFAR-10} datasets, the discarded image count remains relatively stable until a high threshold value is surpassed, while for \textit{CIFAR-100}, it starts to increase exponentially even at relatively low threshold values.
The paper's findings emphasize the significance of the Dynamic Sample Filtering technique in enhancing the Classification Accuracy Score (CAS). However, it is crucial to cautiously validate the threshold value to avoid performance degradation. In cases where the optimal value of this parameter has not yet been determined, we recommend utilizing a value of 0.0.

% \newpage
\begin{figure}[!h]
    \centering
\includegraphics[width=0.8\textwidth,height=0.2\textheight]{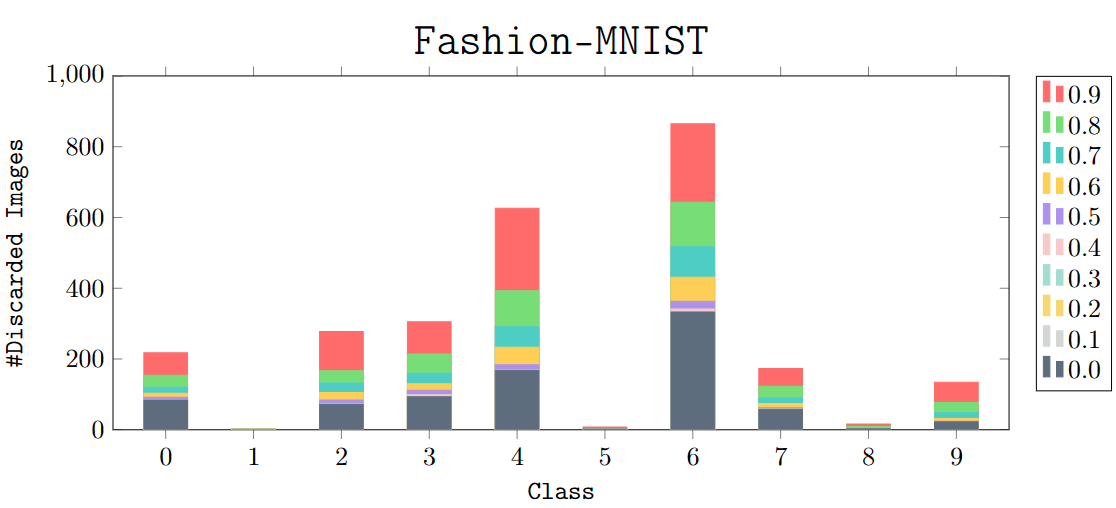}
    \caption{The relationship between the filtering threshold and the number of images discarded for the Fashion-MNIST dataset.}
    \label{fig:filterfmnist}
\end{figure}

\begin{figure}[!h]
    \centering
    \includegraphics[width=0.8\textwidth,height=0.2\textheight]{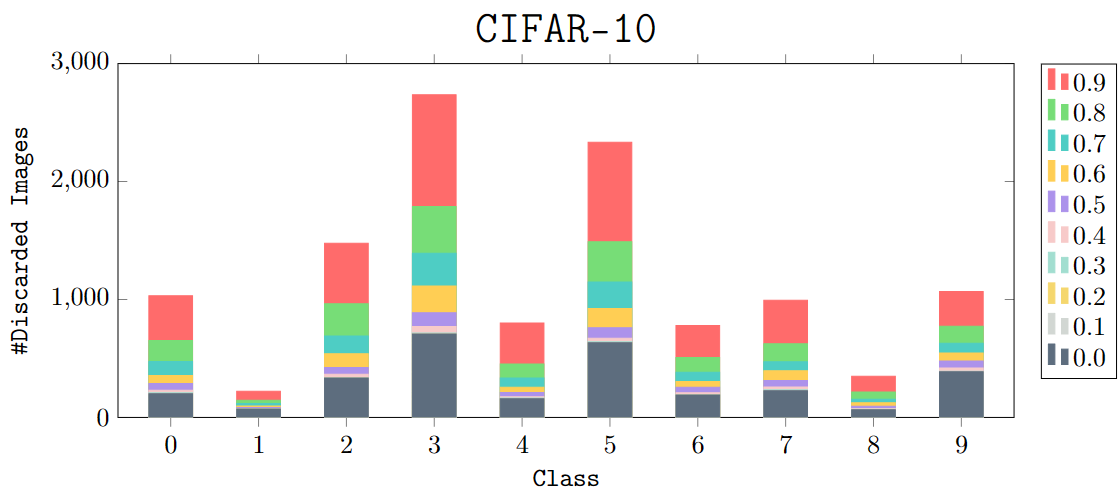}
    \caption{The relationship between the filtering threshold and the number of images discarded for the CIFAR10 dataset.}
    \label{fig:filtercifar10}
\end{figure}

\begin{figure}[!h]
    \centering
    \includegraphics[width=0.8\textwidth,height=0.2\textheight]{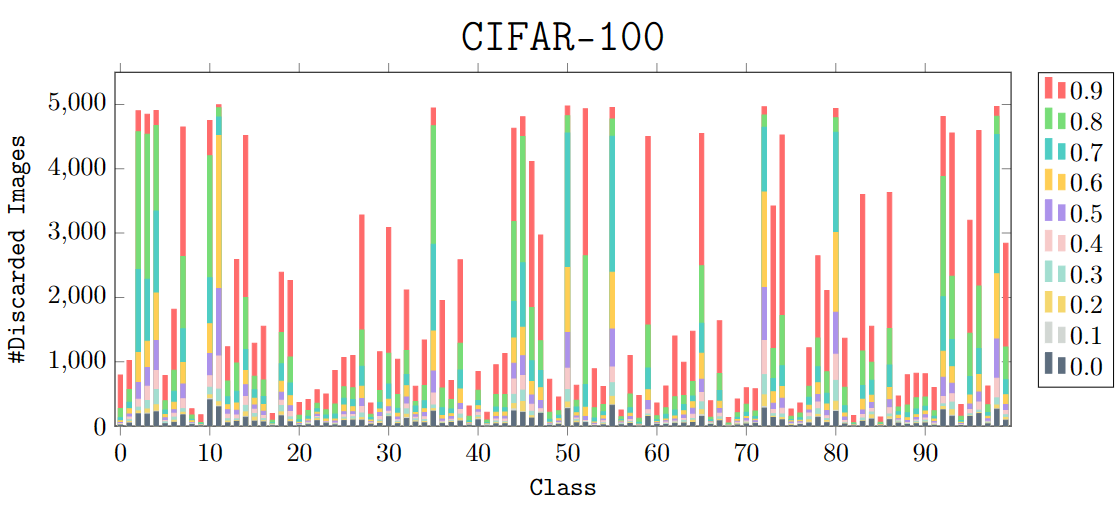}
    \caption{The relationship between the filtering threshold and the number of images discarded for the CIFAR100 dataset.}
    \label{fig:filtercifar100}
\end{figure}

\newpage
\section*{Expansion Trick}
The Expansion Trick involves expanding the input noise space instead of truncating it. This is achieved by sampling from a normal distribution with a higher standard deviation than that used during model training. By broadening the diversity of the input noise space, our approach encourages the generative model to explore underrepresented regions encountered less frequently during training. Consequently, it facilitates the generation of more diverse and novel images, a desirable outcome in scenarios prioritizing diversity over visual fidelity.
However, as anticipated, the increased standard deviation of the input noise distribution adversely impacts the quality of individual samples, as shown in Figure~\ref{fig:expansion_trick_example}. Hence, the effectiveness of the Expansion Trick is enhanced when employed in conjunction with sample filtering techniques. This helps mitigate the negative effects of reduced sample quality by selecting only the most pertinent samples for training the classifier.

\begin{figure}[!h]
    \centering
    \includegraphics[width=0.166\textwidth]{images/Method/Expansion Trick/cifar10_stddev1.0_truck__bad.png}\hfill
    \includegraphics[width=0.166\textwidth]{images/Method/Expansion Trick/cifar10_stddev1.2_truck__bad.png}\hfill
    \includegraphics[width=0.166\textwidth]{images/Method/Expansion Trick/cifar10_stddev1.4_truck__bad.png}\hfill
    \includegraphics[width=0.166\textwidth]{images/Method/Expansion Trick/cifar10_stddev1.6_truck__bad.png}\hfill
    \includegraphics[width=0.166\textwidth]{images/Method/Expansion Trick/cifar10_stddev1.8_truck__bad.png}\hfill
    \includegraphics[width=0.166\textwidth]{images/Method/Expansion Trick/cifar10_stddev2.0_truck__bad.png}\\
    \includegraphics[width=0.166\textwidth]{images/Method/Expansion Trick/cifar10_stddev1.0_truck__good.png}\hfill
    \includegraphics[width=0.166\textwidth]{images/Method/Expansion Trick/cifar10_stddev1.2_truck__good.png}\hfill
    \includegraphics[width=0.166\textwidth]{images/Method/Expansion Trick/cifar10_stddev1.4_truck__good.png}\hfill
    \includegraphics[width=0.166\textwidth]{images/Method/Expansion Trick/cifar10_stddev1.6_truck__good.png}\hfill
    \includegraphics[width=0.166\textwidth]{images/Method/Expansion Trick/cifar10_stddev1.8_truck__good.png}\hfill
    \includegraphics[width=0.166\textwidth]{images/Method/Expansion Trick/cifar10_stddev2.0_truck__good.png}\hfill
    %\vspace{-30pt}
    %\caption[Expansion Trick Example]{Images sampled for class label “Truck”, with standard deviation ranging from 1.0 to 2.0 with increments of 0.2 (fixed seed).}
    \caption[Expansion Trick Example]{Images sampled for class label “Truck”, with standard deviation ranging from 1.0 to 2.0 with increments of 0.2 (fixed seed). Top: image for which a higher stddev degrades the quality, so it will most likely be filtered. Bottom: image for which a higher stddev increases diversity without reducing quality.}
    \label{fig:expansion_trick_example}
    %\vspace{-10pt}
\end{figure}

% \newpage
\section*{Evaluation Metrics}
% We conducted an investigation to determine whether a correlation exists between the Classification Accuracy Score (CAS) and commonly used evaluation metrics for assessing generative models. We present the CAS trends in relation to each specific metric, with a "training checkpoint" referring to an EMA version of the generator saved at a particular epoch.
% The CAS was compared with the Inception Score (IS), Fréchet Inception Distance (FID), and Kernel Inception Distance (KID). However, as observed in Figures~\ref{fig:cifar10metrics} and ~\ref{fig:cifar100metrics}, there is no apparent correlation between these metrics and the CAS. This lack of correlation can be attributed to the fact that traditional metrics fail to capture all aspects of the quality of generated samples that are pertinent to classification tasks. For instance, a sample may possess a low FID score but still be classified incorrectly, indicating its limited utility for downstream tasks. Similarly, the CAS may not encompass all aspects of the diversity and richness of generated samples that hold relevance for other objectives, such as artistic image synthesis.
We investigated the potential correlation between the Classification Accuracy Score (CAS) and commonly utilized evaluation metrics for assessing generative models. Our analysis includes the CAS trends in relation to each specific metric, with "training checkpoints" referring to EMA versions of the generator saved at specific epochs.
The CAS was compared against the Inception Score (IS), Fréchet Inception Distance (FID), and Kernel Inception Distance (KID). However, as evidenced in Figures~\ref{fig:cifar10metrics} and ~\ref{fig:cifar100metrics}, no apparent correlation was found between these metrics and the CAS. This lack of correlation can be attributed to the limitations of traditional metrics in capturing all facets of sample quality relevant to classification tasks. For instance, a sample with a low FID score may still be classified incorrectly, indicating its limited usefulness for downstream applications. Likewise, the CAS may not fully encompass the diversity and richness of generated samples that are significant for other objectives, such as artistic image synthesis.

% \newpage
\begin{figure}[p]
    \centering
    \includegraphics[width=1.\textwidth]{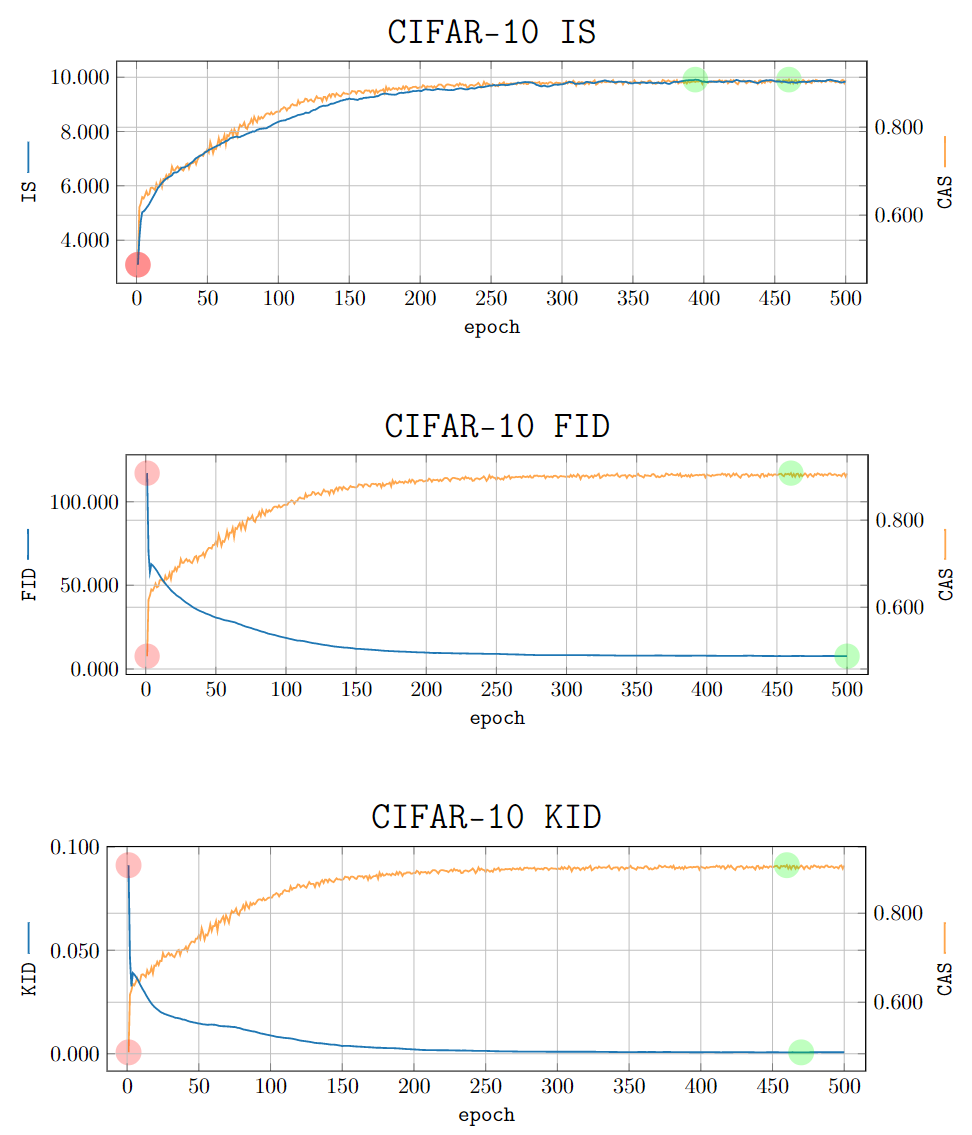}  
    \caption{The comparison of the Classification Accuracy Score (CAS) with Inception Score (IS), Fréchet Inception Distance (FID), and Kernel Inception Distance (KID) for each checkpoint (CIFAR-10 dataset).}
    \label{fig:cifar10metrics}
\end{figure}

% \newpage
\begin{figure}[p]
    \centering
    \includegraphics[width=1.\textwidth]{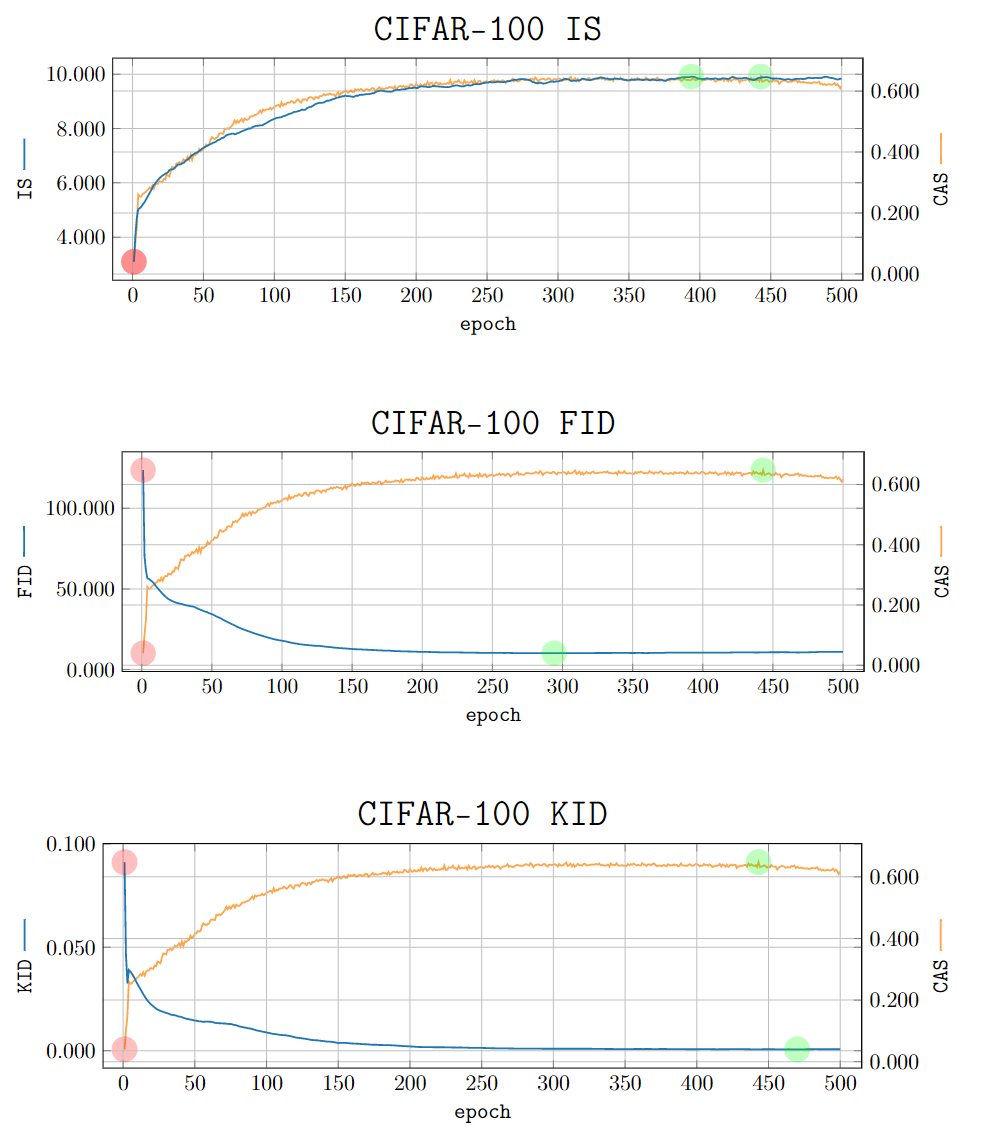}
    \caption{The comparison of the Classification Accuracy Score (CAS) with Inception Score (IS), Fréchet Inception Distance (FID), and Kernel Inception Distance (KID) for each checkpoint (CIFAR-100 dataset).}
    \label{fig:cifar100metrics}
\end{figure}

\newpage
\section*{Datasets t-SNE Embeddings}
% In Figures~\ref{fig:tsne_fm_unfiltered},~\ref{fig:tsne_fm_filtered},~\ref{fig:tsne_fm_optimal},~\ref{fig:tsne_cifar10_unfiltered},~\ref{fig:tsne_cifar10_filtered},~\ref{fig:tsne_cifar10_optimal},~\ref{fig:tsne_cifar100_unfiltered},~\ref{fig:tsne_cifar100_filtered},~\ref{fig:tsne_cifar100_optimal} we show t-SNE embedding of all the classes for \textit{Fashion-MNIST} and \textit{CIFAR-10} datsets, and of 10 classes for \textit{CIFAR-100}. The t-SNE visualizations are generated with the embeddings of these images in the feature space of the baseline classifier trained on the real training sets, i.e., the ResNet-20 used in all our experiments. The “features space” of a CNN classifier refers to the output of the convolutional part of the network. In the case of the ResNet-20 used in our experiments, the feature space is the output of the last AveragePooling2D layer before the fully connected layers. This layer outputs a tensor containing a set of high-level features learned by the network from the input images. These features can be seen as a compressed representation of the input images that captures the most relevant patterns and structures for the classification task. By using the feature space as the basis for the t-SNE embeddings, we can visualize the distribution of images in a reduced-dimensional space that reflects the similarities and differences between their high-level features. This allows us to gain insights into how the classifier is grouping images from different classes, and to assess the quality of the learned features in terms of their discriminative power.
Figures~\ref{fig:tsne_fm_unfiltered},~\ref{fig:tsne_fm_filtered},~\ref{fig:tsne_fm_optimal},~\ref{fig:tsne_cifar10_unfiltered},~\ref{fig:tsne_cifar10_filtered},~\ref{fig:tsne_cifar10_optimal},~\ref{fig:tsne_cifar100_unfiltered},~\ref{fig:tsne_cifar100_filtered},~\ref{fig:tsne_cifar100_optimal} present t-SNE embeddings of all classes for the \textit{Fashion-MNIST} and \textit{CIFAR-10} datasets, and 10 classes for \textit{CIFAR-100}. These t-SNE visualizations are generated using the embeddings of these images in the feature space of the baseline classifier, specifically the ResNet-20 employed in all our experiments.
The feature space of a CNN classifier refers to the output of the network's convolutional component. For our experiments utilizing ResNet-20, the feature space corresponds to the output of the last AveragePooling2D layer prior to the fully connected layers. This layer produces a tensor comprising high-level features learned by the network from the input images. These features serve as a condensed representation of the input images, capturing the most relevant patterns and structures for the classification task.
By leveraging the feature space as the foundation for t-SNE embeddings, we visualize the distribution of images in a lower-dimensional space that reflects the similarities and dissimilarities among their high-level features. This approach allows us to gain insights into how the classifier clusters images from different classes and assess the quality of the learned features in terms of their discriminative power.

\begin{figure}[!b]
    \includegraphics[width=\textwidth,height=0.5\textheight]{images/Method/tsne/fashionmnist_unfiltered_stddev1.0_tsne.png}
    \caption[t-SNE Fashion-MNIST Unfiltered]{t-SNE embedding of images from \textit{Fashion-MNIST} classes, embedded in the feature space of the baseline ResNet-20 classifier. We use 500 images each from the train and test sets, along with 500 images each generated with BigGAN. No post-processing techniques have been applied.}
    \label{fig:tsne_fm_unfiltered}
\end{figure}

\clearpage
\begin{figure}[p]
    \includegraphics[width=\textwidth,height=0.5\textheight]{images/Method/tsne/fashionmnist_filter0.0_stddev1.0_tsne.png}
    \caption[t-SNE Fashion-MNIST Filtered]{t-SNE embedding of images from \textit{Fashion-MNIST} classes, embedded in the feature space of the baseline ResNet-20 classifier. We use 500 images each from the train and test sets, along with 500 images each generated with BigGAN. Dynamic Sample Filtering has been applied with a threshold of 0.0.}
    \label{fig:tsne_fm_filtered}
\end{figure}

\begin{figure}[p]
    \includegraphics[width=\textwidth,height=0.5\textheight]{images/Method/tsne/fashionmnist_filter0.0_stddev2.0_tsne.png}
    \caption[t-SNE Fashion-MNIST Optimal]{t-SNE embedding of images from \textit{Fashion-MNIST} classes, embedded in the feature space of the baseline ResNet-20 classifier. We use 500 images each from the train and test sets, along with 500 images each generated with BigGAN. Dynamic Sample Filtering and Expansion Trick have been applied with the optimal hyperparameters.}
    \label{fig:tsne_fm_optimal}
\end{figure}

%%%%% CIFAR-10 %%%%%
\clearpage
\begin{figure}[p]
    \includegraphics[width=\textwidth,height=0.5\textheight]{images/Method/tsne/cifar10_unfiltered_stddev1.0_tsne.png}
    \caption[t-SNE Cifar-10 Unfiltered]{t-SNE embedding of images from \textit{CIFAR-10} classes, embedded in the feature space of the baseline ResNet-20 classifier. We use 500 images each from the train and test sets, along with 500 images each generated with BigGAN. No post-processing techniques have been applied.}
    \label{fig:tsne_cifar10_unfiltered}
\end{figure}

\begin{figure}[p]
    \includegraphics[width=\textwidth,height=0.5\textheight]{images/Method/tsne/cifar10_filter0.0_stddev1.0_tsne.png}
    \caption[t-SNE Cifar-10 Filtered]{t-SNE embedding of images from \textit{CIFAR-10} classes, embedded in the feature space of the baseline ResNet-20 classifier. We use 500 images each from the train and test sets, along with 500 images each generated with BigGAN. Dynamic Sample Filtering has been applied with a threshold of 0.0.}
    \label{fig:tsne_cifar10_filtered}
\end{figure}

\begin{figure}[p]
    \includegraphics[width=\textwidth,height=0.5\textheight]{images/Method/tsne/cifar10_filter0.3_stddev1.6_tsne.png}
    \caption[t-SNE Cifar-10 Optimal]{t-SNE embedding of images from \textit{CIFAR-10} classes, embedded in the feature space of the baseline ResNet-20 classifier. We use 500 images each from the train and test sets, along with 500 images each generated with BigGAN. Dynamic Sample Filtering and Expansion Trick have been applied with the optimal hyperparameters.}
    \label{fig:tsne_cifar10_optimal}
\end{figure}

%%%%% CIFAR-100 %%%%%
\clearpage
\begin{figure}[p]
    \includegraphics[width=\textwidth,height=0.5\textheight]{images/Method/tsne/cifar100_unfiltered_stddev1.0_tsne.png}
    \caption[t-SNE Cifar-100 Unfiltered]{t-SNE embedding of images from \textit{CIFAR-100} classes, embedded in the feature space of the baseline ResNet-20 classifier. We use 500 and 100 images each from the train and test sets respectively, along with 500 images each generated with BigGAN. No post-processing techniques have been applied.}
    \label{fig:tsne_cifar100_unfiltered}
\end{figure}

\begin{figure}[p]
    \includegraphics[width=\textwidth,height=0.5\textheight]{images/Method/tsne/cifar100_filter0.0_stddev1.0_tsne.png}
    \caption[t-SNE Cifar-100 Filtered]{t-SNE embedding of images from \textit{CIFAR-100} classes, embedded in the feature space of the baseline ResNet-20 classifier. We use 500 and 100 images each from the train and test sets respectively, along with 500 images each generated with BigGAN. Dynamic Sample Filtering has been applied with a threshold of 0.0.}
    \label{fig:tsne_cifar100_filtered}
\end{figure}

\begin{figure}[p]
    \includegraphics[width=\textwidth,height=0.5\textheight]{images/Method/tsne/cifar100_filter0.1_stddev1.7_tsne.png}
    \caption[t-SNE Cifar-100 Optimal]{t-SNE embedding of images from \textit{CIFAR-100} classes, embedded in the feature space of the baseline ResNet-20 classifier. We use 500 and 100 images each from the train and test sets respectively, along with 500 images each generated with BigGAN. Dynamic Sample Filtering and Expansion Trick have been applied with the optimal hyperparameters.}
    \label{fig:tsne_cifar100_optimal}
\end{figure}
